# Supplementary material for: Diffusion-based mass map reconstruction from weak lensing data
Source: arXiv:2502.04158 source file (2025-02-06)
Supplement: Supplementary file 1 [file dps_extensions.tex]

\section{Extensions to DPS}\label{sec:dps_extensions}

\subsection{Step-wise Triple-Consistent Diffusion Sampling for Inverse Problems (SITCOM)}\label{ssec:sitcom}

The other method we use is the Step-wise Triple-Consistent Diffusion Sampling for Inverse Problems (SITCOM) algorithm \cite{sitcom}. In this algorithm, they impose three conditions in the posterior sampling (\red{The following text is taken from the SITCOM paper}): 

\begin{itemize}
    \item \textbf{Measurement Consistency}: The reconstruction $\hat{\mvec{x}}^{'}_0$ is consistent with the measurements This means that $A(\hat{\mvec{x}}^{'}_0) \approx \mvec{d}$.
    \item \textbf{Backward Consistency}: The reconstruction $\hat{\mvec{x}}^{'}_0$ is a denoised image produced by the Tweedie network denoiser $f$. More generally, we define the backward consistency to include any form of DM network regularization (e.g., using the DM probability-flow (PF) ODE [32]) applied to $\hat{\mvec{x}}^{'}_0$.
    \item \textbf{Forward Consistency}: The pre-trained DM network $\epsilon_{\theta}$ is provided with in-distribution inputs with high probability. To ensure this, we apply the resampling formula in (8) and enforce that $\mvec{v}^t$ remains close to $\mvec{x}_t$.
\end{itemize}
In order to do this, they follow a three-step procedure, 
\begin{itemize}
    \item \textbf{Step 1}: Perform an optimization over the following objective function, 
    \begin{equation}\label{eqn:sitcom_optimzation}
        L(\mvec{v}_t) = \log L(f(\mvec{v}_t)) + \lambda |\mvec{x}_t - \mvec{v}_t|^2,
    \end{equation}
    where $f(\mvec{v}_t)$ is the Tweedie prediction, 
    \begin{equation}
        f(\mvec{v}_t) = \frac{1}{\bar{\alpha}_t}\bigg[\mvec{v}_t - \sqrt{1-\bar{\alpha}_t} \mvec{\epsilon}(\mvec{v}_t, t)\bigg],
    \end{equation}
    and $\log L$ is the likelihood. The second term in the equation \eqref{eqn:sitcom_optimzation} is a regularization term that ensures that the prediction is not far away from the distribution where the diffusion model is trained. 
    \item \textbf{Step 2}: Tweedie prediction from the optimization result, $\hat{\mvec{v}}_t$, 
    \begin{equation}
        \hat{\mvec{x}}_t = f(\hat{\mvec{v}}_t, t).
    \end{equation}
    \item \textbf{Step 3}: Add stochasticity to the Tweedie prediction,
    \begin{equation}
        \mvec{x}_{t-1} = \sqrt{\bar{\alpha}_{t-1}} \hat{\mvec{x}}_t + \sqrt{1 - \bar{\alpha}_{t-1}} \mvec{\eta}_t,
    \end{equation}
    where, $\mvec{\eta}_t \sim \mathcal{N}(0,\mathbf{I})$.
\end{itemize}

\subsection{Decoupled Annealed Posterior Sampling}\label{ssec:daps}

The decoupled annealed posterior sampling algorithm (DAPS) \cite{daps} involves a two-step sampling process:

\begin{enumerate}
    \item \textbf{Step 1}: Sample $\mvec{x}_{0|\mvec{d}} \sim p(\mvec{x}_0|\mvec{d}, \mvec{x}_t)$.
    \item \textbf{Step 2}: Sample 
    \begin{equation}    
    \mvec{x}_{t-1} \sim p(\mvec{x}_{t-1}|\mvec{x}_{0|\mvec{d}}) = \mathcal{N}(\mvec{x}_{0|\mvec{d}}, \sigma^2_{t-1}).
    \end{equation}
\end{enumerate}

The second step is simple and it just requires the noise used for the forward diffusion process. 

To simplify the first step, we use Bayes theorem to write, 
\begin{equation}\label{eqn:x0_posterior}
    p(\mvec{x}_0|\mvec{d}, \mvec{x}_t) = p(\mvec{d}|\mvec{x}_0)p(\mvec{x}_0|\mvec{x}_t).
\end{equation}
The first term on the RHS is likelihood. The second term is more complicated, but the paper simplifies it as a Gaussian, 
\begin{equation}
    p(\mvec{x}_0|\mvec{x}_t)=\mathcal{N}(\hat{\mvec{x}}_0(\mvec{x}_t, t), r^2_t).
\end{equation}
The mean of the posterior, $p(\mvec{x}_0|\mvec{x}_t)$ is the Tweedie formula, equation \eqref{eqn:tweedie}. The variance $r^2_t$ is not straightforward, and in \cite{daps}, they determine this variance ``using heuristics". I think we can determine the variance by sampling the unconditioned diffusion model. 

Although this simplifies the posterior, \eqref{eqn:x0_posterior}, sampling from this posterior is not straightforward. In \cite{daps}, they use Langevin sampling to sample from this posterior. We might also be able to use simpler methods to sample from this posterior. The posterior in this case is very similar to the case of sampling from a Wiener posterior, where there are well developed methods for sampling from this posterior.
